# Supplementary material for: Defect Physics of Pseudo-cubic Mixed Halide Lead Perovskites from First Principles
Source: arXiv:1908.05585 ancillary file (2019-08-15)
Supplement: Supplementary file 1 [file Supplementary_Information.pdf]

*Supporting Information*

# Defect Physics of Pseudo-cubic Mixed Halide Lead Perovskites from First Principles

Arun Mannodi-Kanakkithodi, Ji-Sang Park, Alex B. F. Martinson and Maria K.Y. Chan

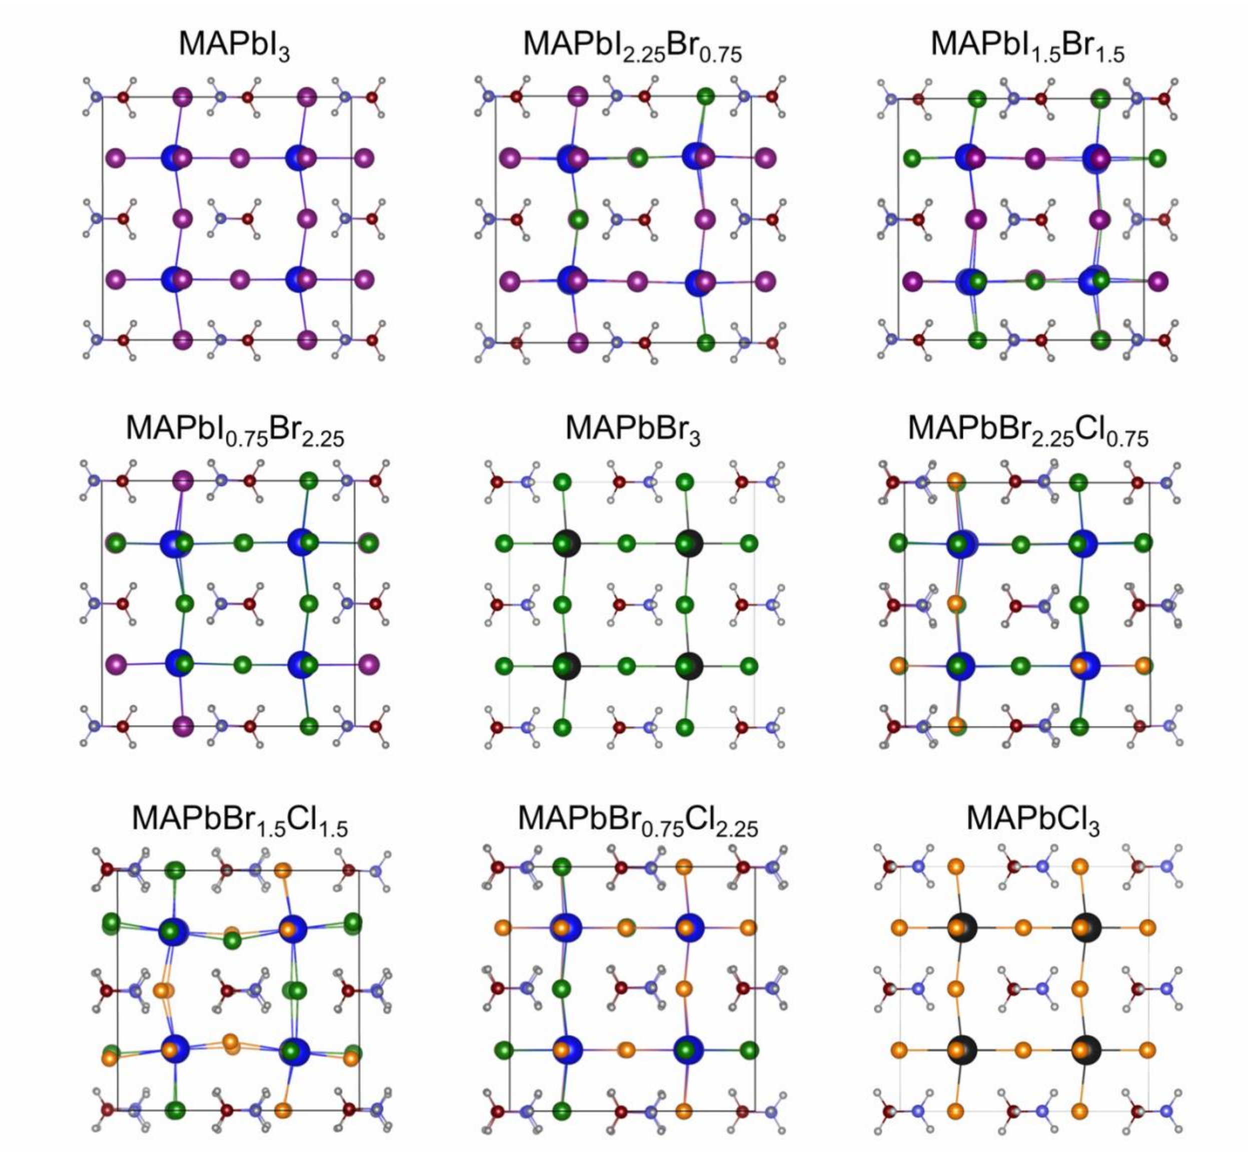


**Fig. SI1.** Structures of all 9 perovskites. Pb atoms are in blue, I in magenta, Br in green, Cl in orange, C in maroon, N in purple and H in grey.

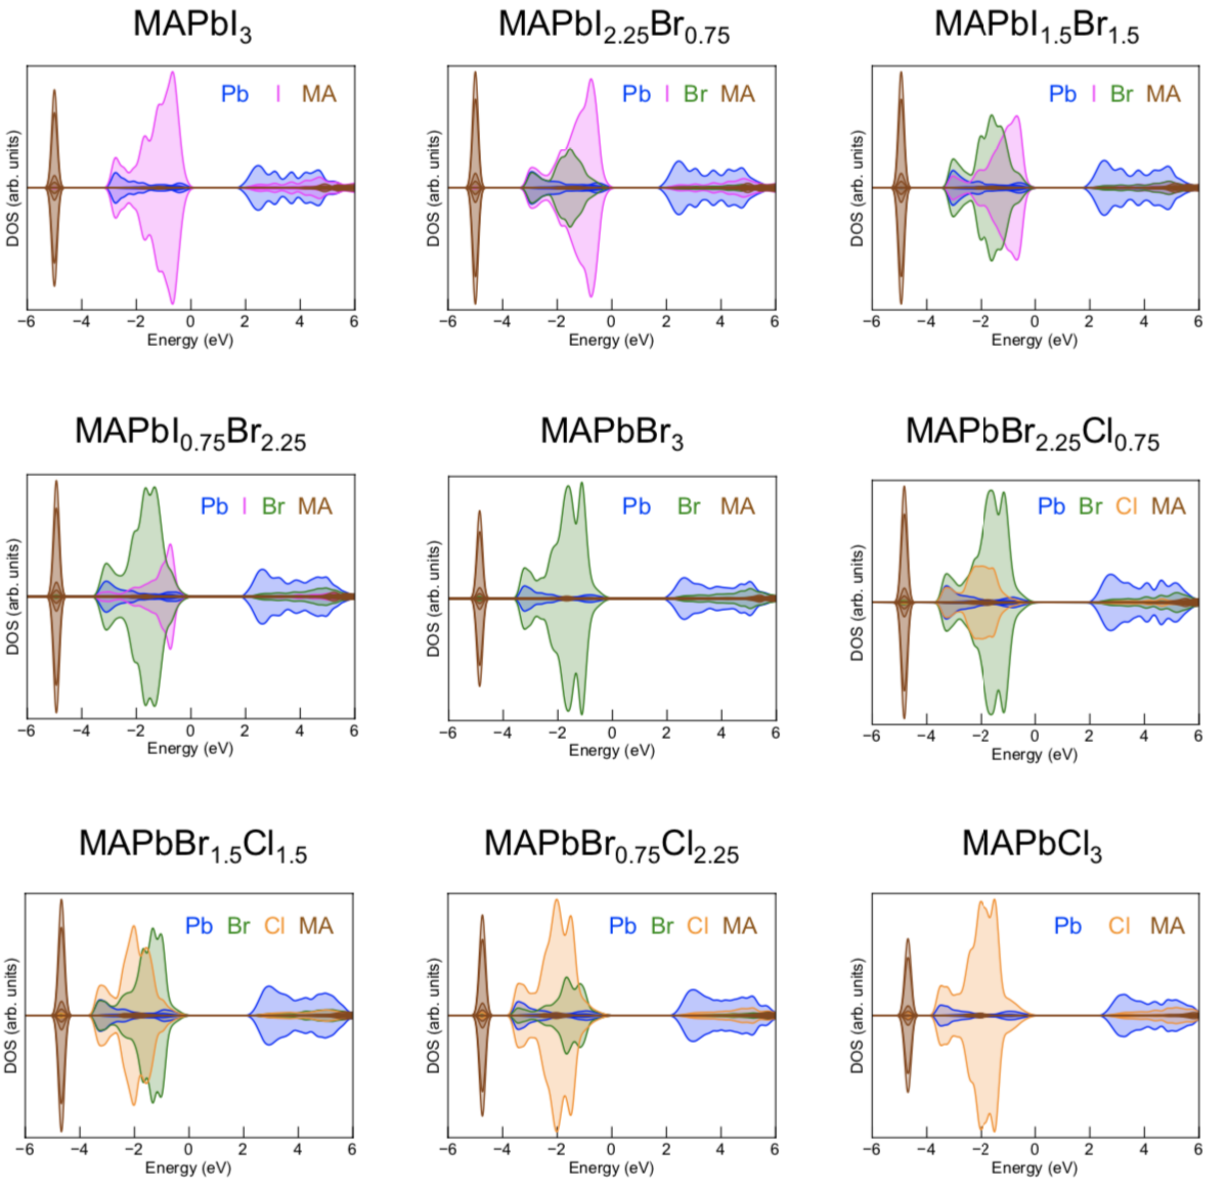


**Fig. SI2.** Computed DOS for all 9 perovskites.

| System | Lattice Constant (Å) | Band Gap (eV) | Mixing energy wrt pure $MAPbX_3$ (meV per f.u.) |
|---|---|---|---|
| $MAPbI_3$ | 6.42 (6.3 [a,b]) | 1.80 (1.58 [f]) | 0 |
| $MAPbI_{2.25}Br_{0.75}$ | 6.35 (~ 6.2 [e]) | 1.83 (~1.7 [f]) | 15.55 |
| $MAPbI_{1.5}Br_{1.5}$ | 6.25 (~ 6.1 [e]) | 1.89 (1.86 [f]) | 11.64 |
| $MAPbI_{0.75}Br_{2.25}$ | 6.15 (~ 6 [e]) | 1.92 (~2 [f]) | 10.29 |
| $MAPbBr_3$ | 6.07 (5.95 [c,d]) | 1.97 (2.27 [c]) | 0 |
| $MAPbBr_{2.25}Cl_{0.75}$ | 6.01 (5.9 [d]) | 2.09 (~2.5 [d]) | 12.03 |
| $MAPbBr_{1.5}Cl_{1.5}$ | 5.93 (~ 5.8 [c,d]) | 2.26 (2.52 [c]) | 3.67 |
| $MAPbBr_{0.75}Cl_{2.25}$ | 5.87 (5.75 [d]) | 2.30 (~2.8 [d]) | 13.95 |
| $MAPbCl_3$ | 5.76 (5.7 [d]) | 2.55 (~2.9 [g]) | 0 |

**Table SI-1.** DFT computed lattice constants, band gaps and formation energies (referenced to pure, unmixed halide perovskites) for the 9 perovskites.


a. P.S. Whitfield et al., *Sci Rep.*, 6, 35685 (2016).
b. F.F. Targhi et al., *Results in Physics*, 10, 616-627 (2018).
c. M.D. Sampson et al., *J. Mater. Chem. A*., 5, 3578 (2017).
d. R. Comin et al., *J. Mater. Chem. C.*, 3, 8839 (2015).
e. F. Lehmann et al., *RSC Adv.*, 9, 11151 (2019).
f. L. Gil-Escrig et al., *J. Phys. Chem. Lett.*, 6, 3743-3748 (2015).
g. G. Maculan et al., *J. Phys. Chem. Lett.*, 6, 3781-3786 (2015).

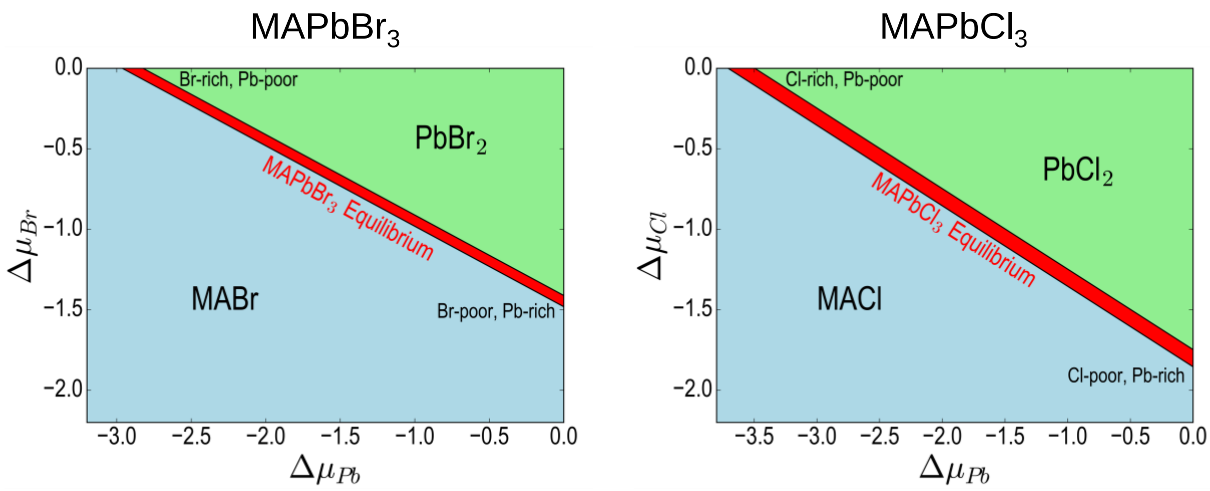


**Fig. SI3.** Calculated chemical ranges of stability for $MAPbBr_3$ and $MAPbCl_3$.

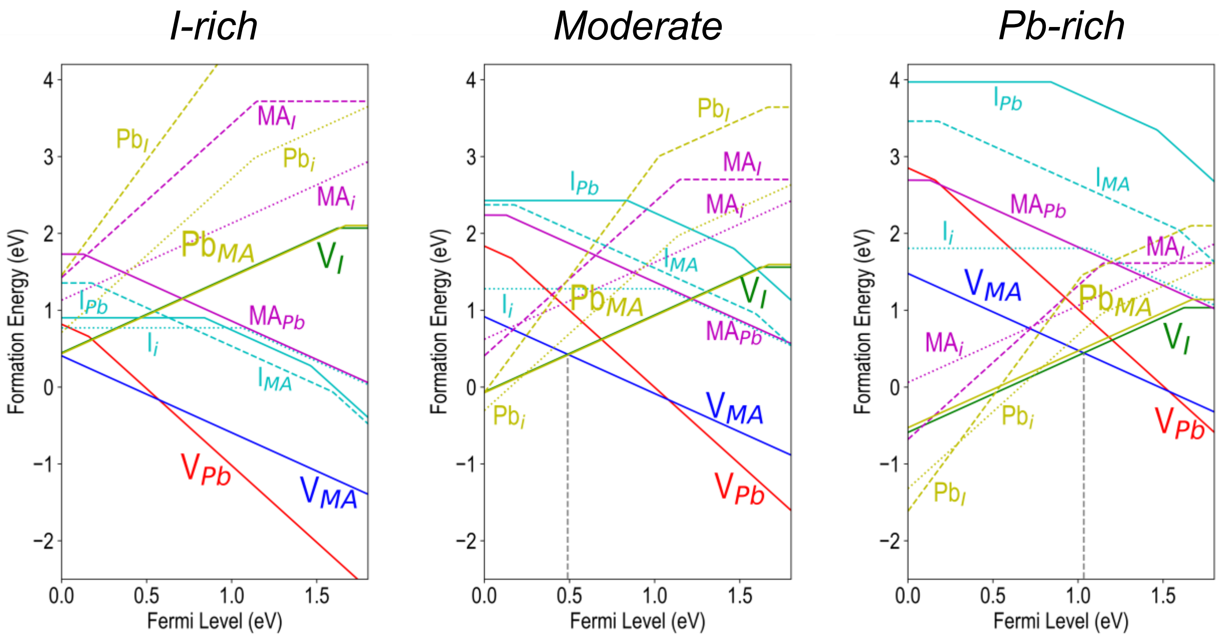


**Fig. SI4.** All native defect formation energies in $MAPbI_3$.

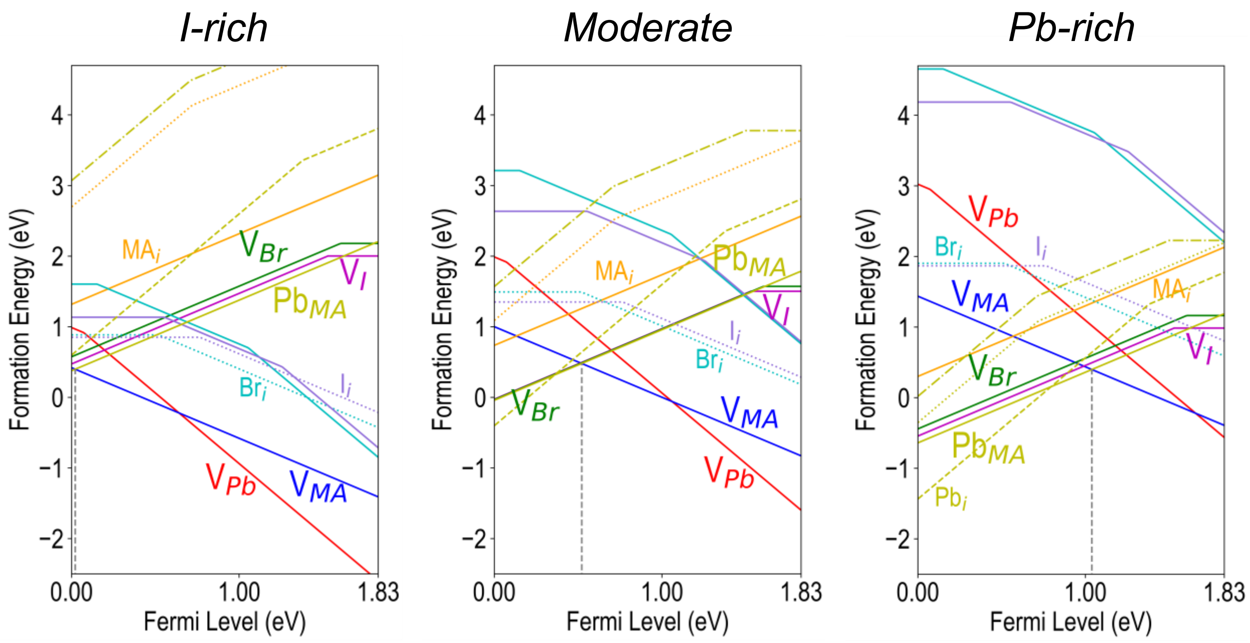


**Fig. SI5.** All native defect formation energies in $MAPbI_{2.25}Br_{0.75}$.

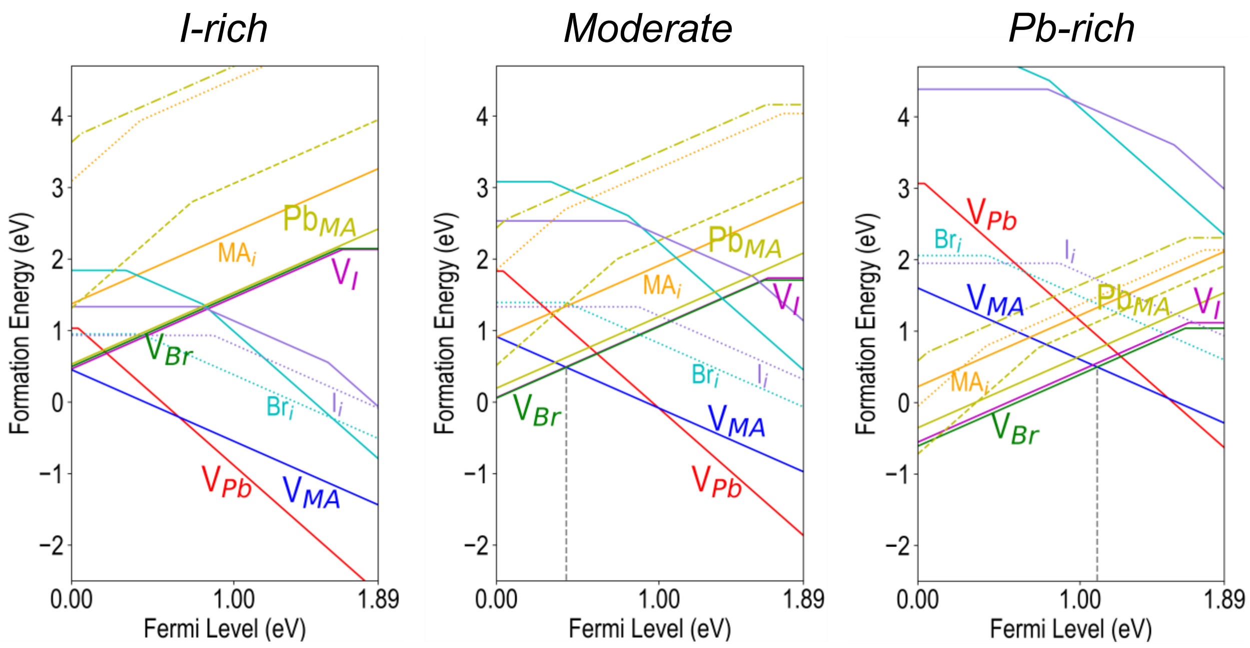


**Fig. SI6.** All native defect formation energies in $MAPbI_{1.5}Br_{1.5}$.

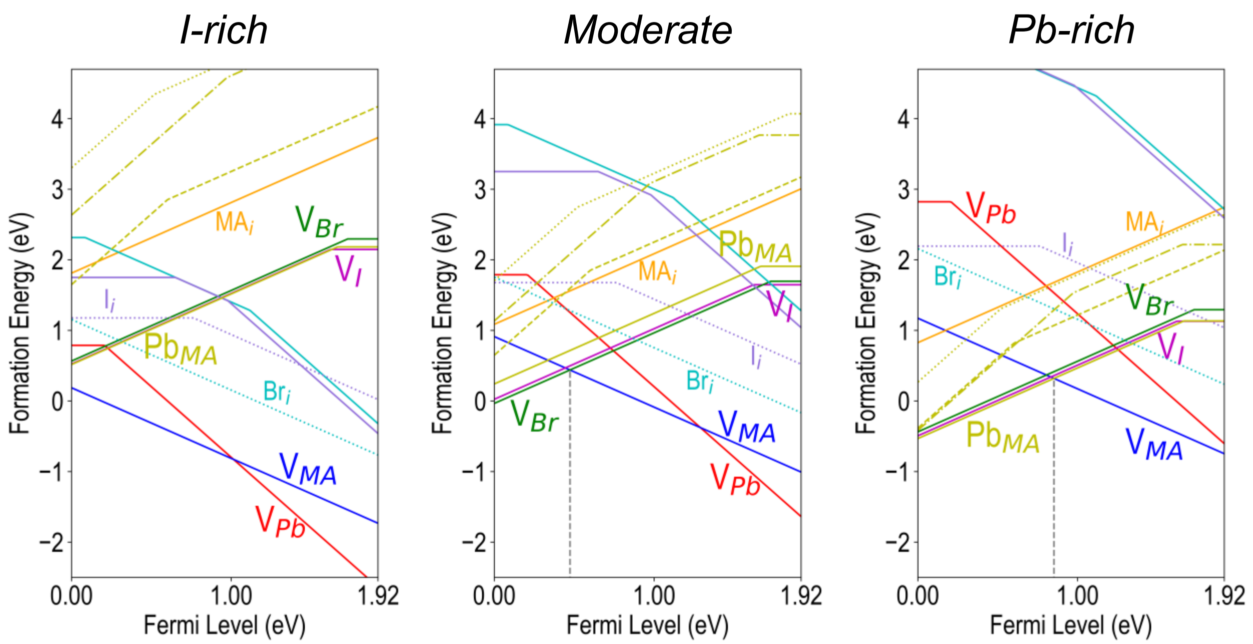


**Fig. SI7.** All native defect formation energies in $MAPbI_{0.75}Br_{2.25}$.

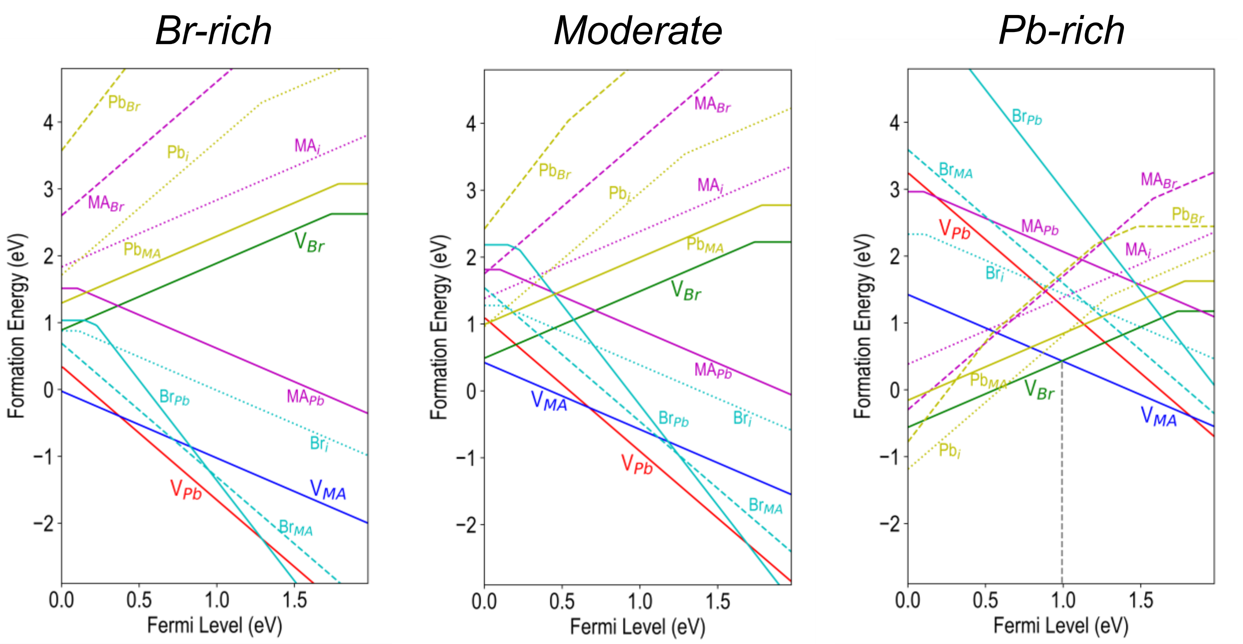


**Fig. SI8.** All native defect formation energies in $MAPbBr_3$.

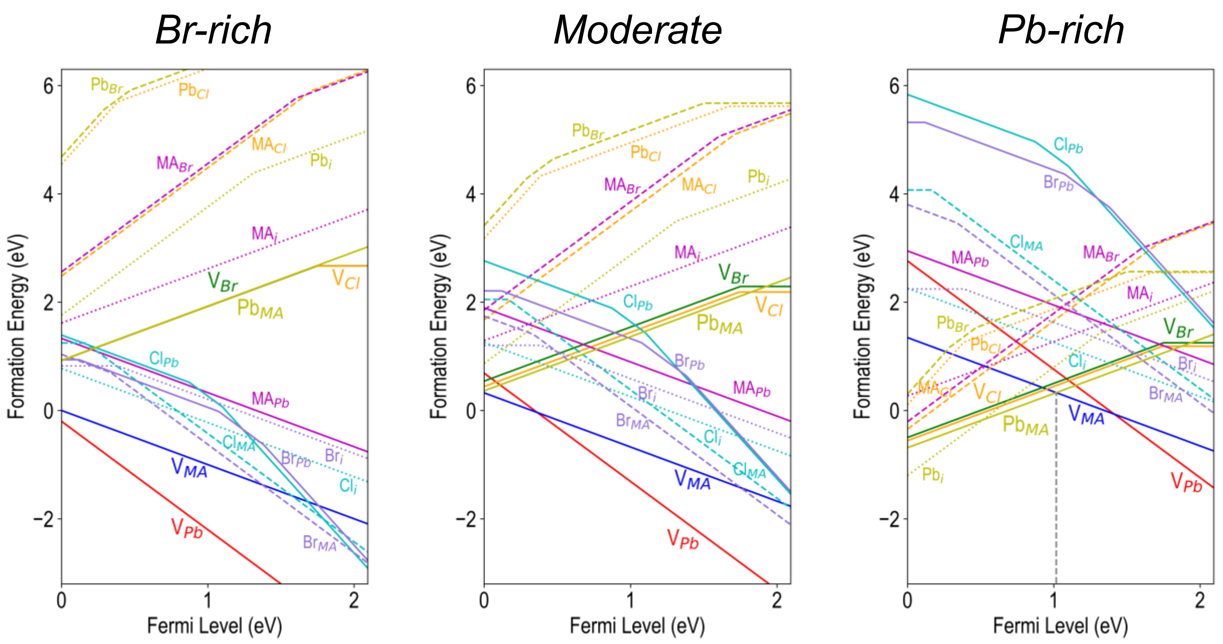


**Fig. SI9.** All native defect formation energies in $MAPbBr_{2.25}Cl_{0.75}$.

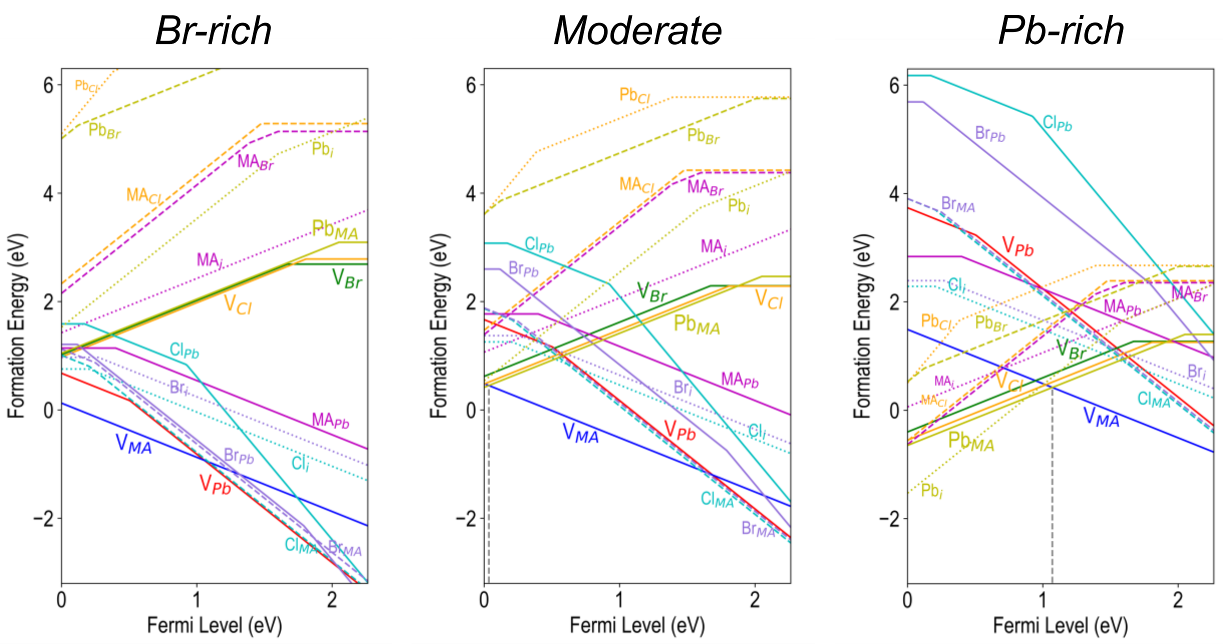


**Fig. SI10.** All native defect formation energies in $MAPbBr_{1.5}Cl_{1.5}$.

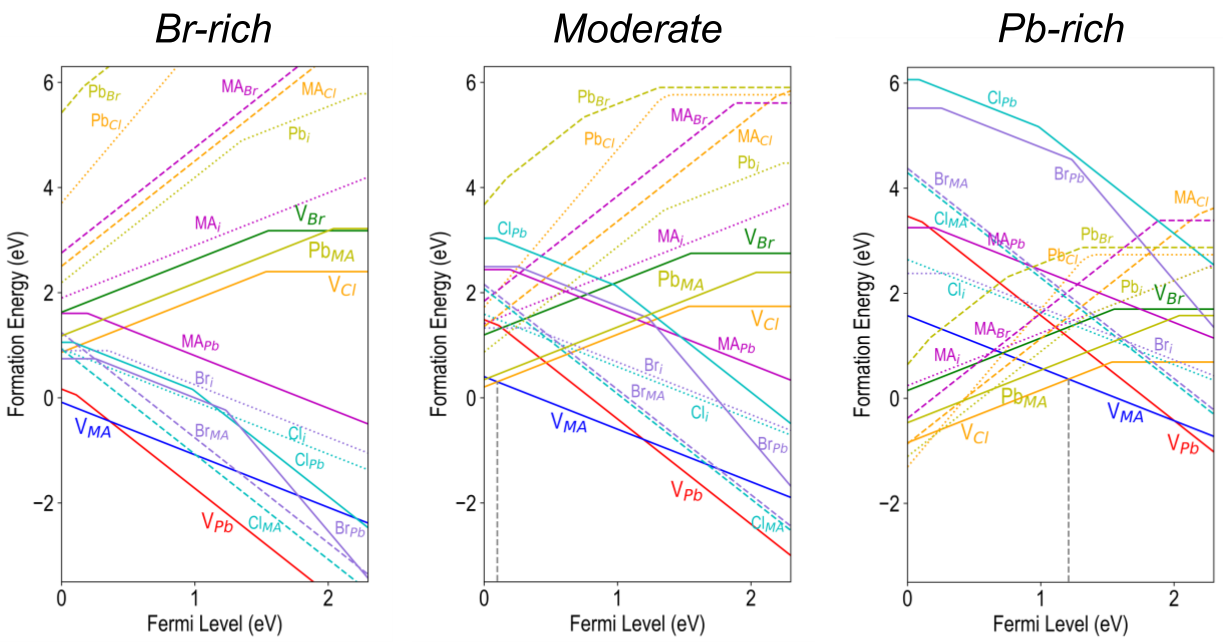


**Fig. SI11.** All native defect formation energies in $MAPbBr_{0.75}Cl_{2.25}$.

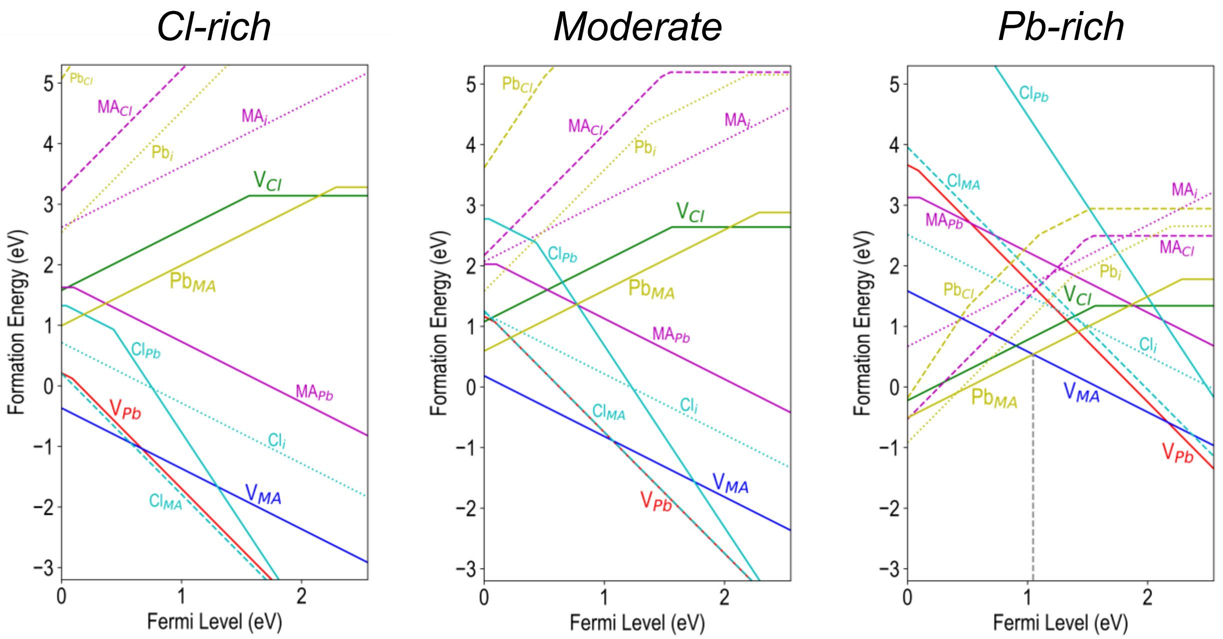


**Fig. SI12.** All native defect formation energies in $MAPbCl_3$.

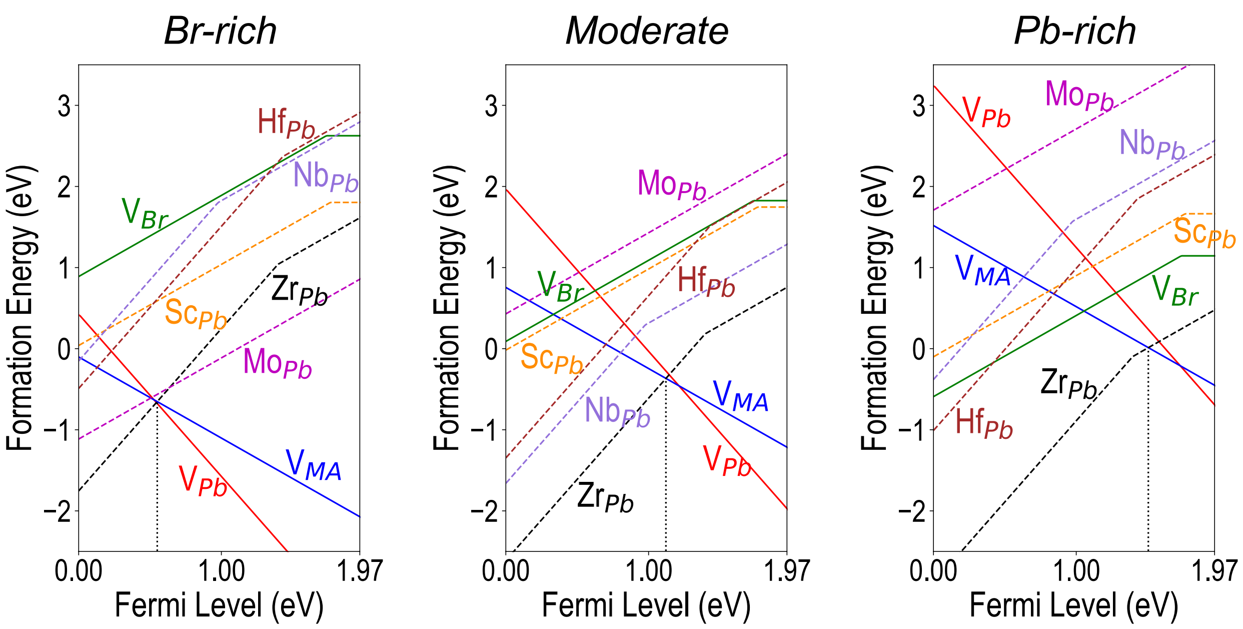


**Fig. SI13.** Computed formation energies for Pb-site substitutional defects in $MAPbBr_3$.
